# Supplementary material for: Femto-Containers: DevOps on Microcontrollers with Lightweight Virtualization & Isolation for IoT Software Modules
Source: arXiv:2106.12553 source file (2021-11-03)
Supplement: Supplementary file 1 [file 4a-bpf-additional-background.tex]

\section{Additional Background on eBPF Virtualization}
The virtual machine operates on 11 registers of 64 bits.
The last register (\texttt{r10}) is a read-only pointer to the beginning of a \SI{512}{\byte} stack.
Interaction with the stack happens via load and store instructions as shown in \autoref{fig:isa}.
% moving values from the registers to the stack and vise versa.
Instructions are divided into an \SI{8}{\bit} opcode, two \SI{4}{\bit} registers: source and destination, an \SI{16}{\bit} offset field and an \SI{32}{\bit} immediate value.
Unused fields in an instruction are set to zero.
Position-independent code is achieved by using the reference in \texttt{r10} and the offset field in the instructions.

\begin{figure}[t]
  \centering
    \includegraphics[width=\columnwidth]{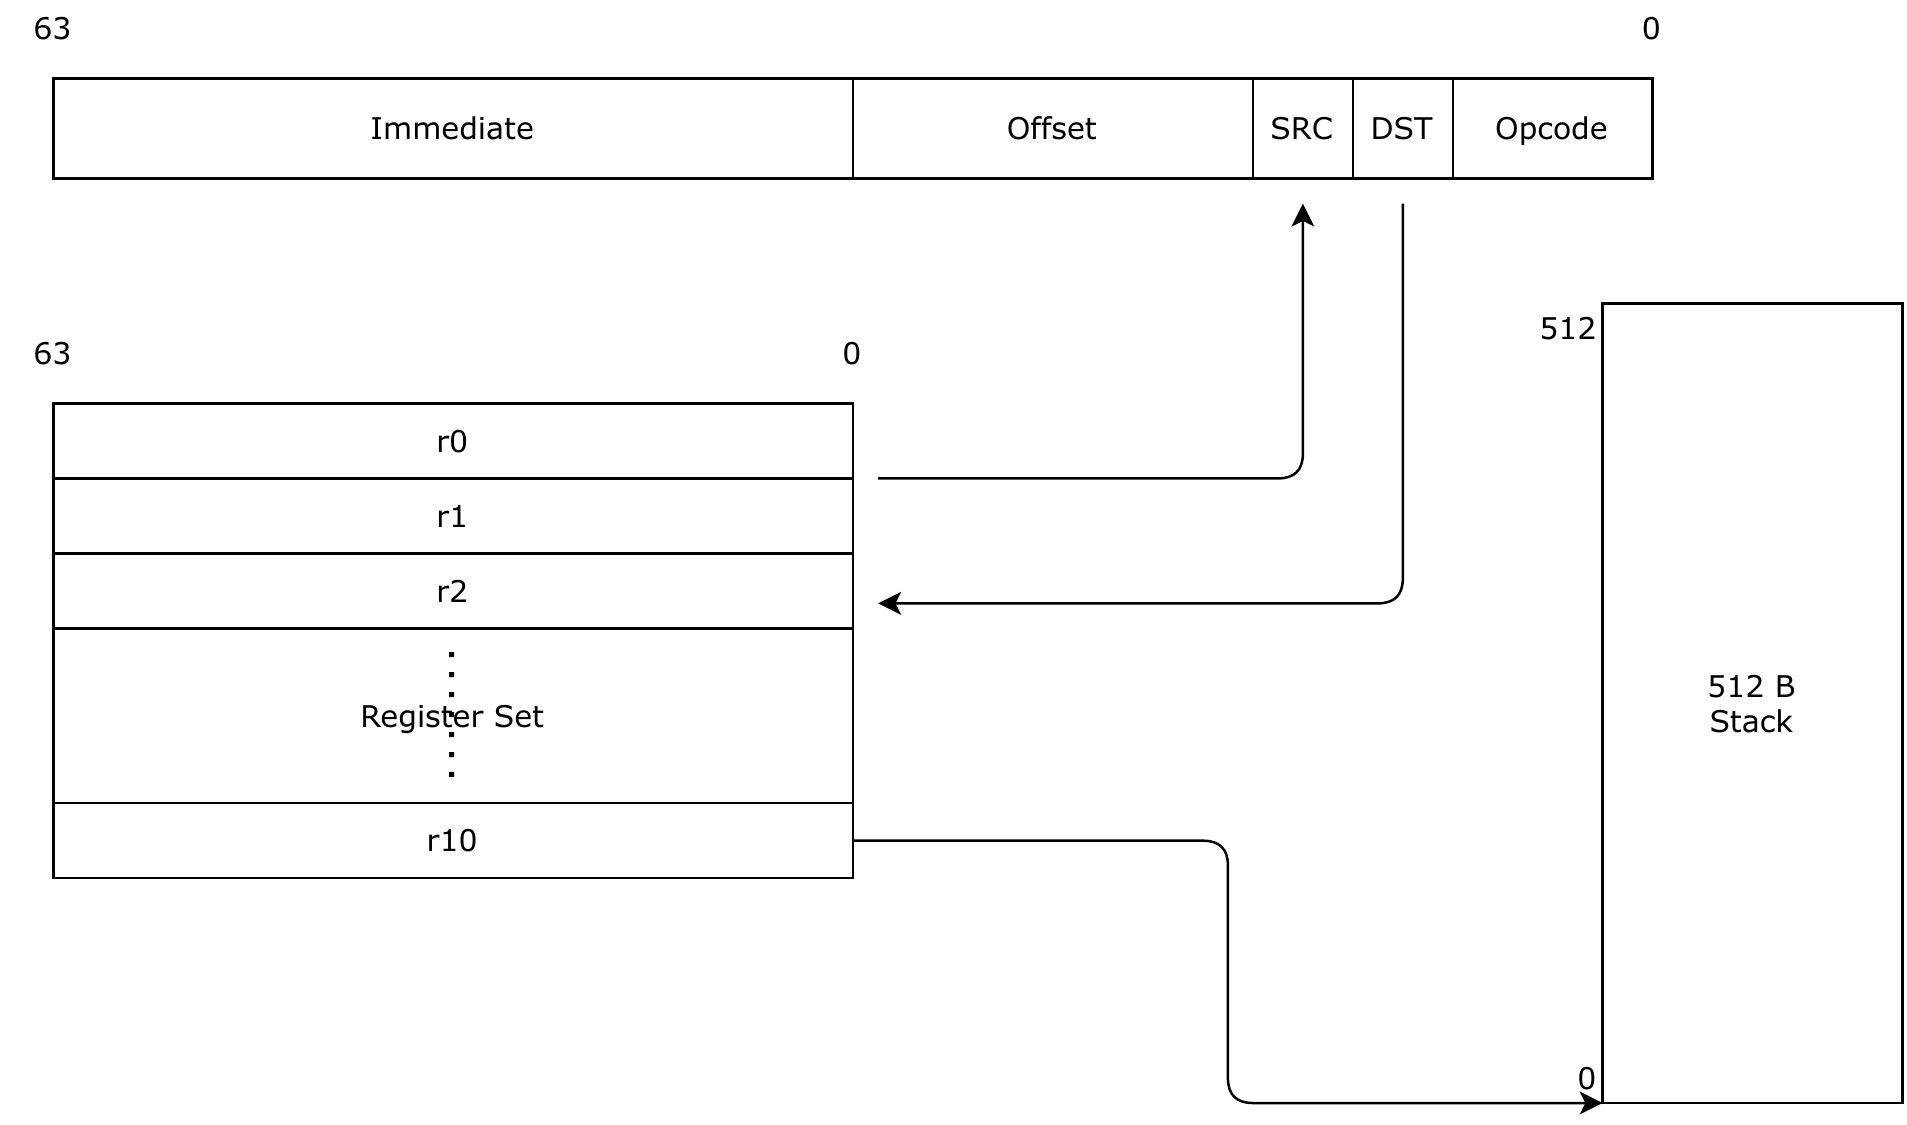}
  \caption{eBPF instructions, registers and stack.}
  \label{fig:isa}
\end{figure}

%Most instruction do not use all fields, the fields not used for an instruction must be zero.
